# Supplementary material for: Non-collinear magnetic structure and multipolar order in Eu$_2$Ir$_2$O$_7$
Source: arXiv:1705.01157 source file (2017-09-28)
Supplement: Supplementary file 1 [file suppl.pdf]

# Supplementary Material of "Non-collinear magnetic structure and multipolar order in $Eu_2Ir_2O_7$"

Yilin Wang,[1] Hongming Weng,[1] Liang Fu,[2] and Xi Dai[1,3]

[1] *Beijing National Laboratory for Condensed Matter Physics, and Institute of Physics, Chinese Academy of Sciences, Beijing 100190, China*
[2] *Department of physics, Massachusetts Institute of Technology, Cambridge, MA 02139, USA*
[3] *Collaborative Innovation Center of Quantum Matter, Beijing 100190, China*

(Dated: September 26, 2017)

## I. COMPUTATIONAL DETAILS

Fig. S1(a) is the crystal structure of $Eu_2Ir_2O_7$. It has a face-centered cubic (FCC) structure with space group $Fd\bar{3}m$, with Ir atoms occupying the $\bar{3}m$ sites. Fig. S1(b) is the Brillouin zone and some high-symmetry $k$-paths of FCC crystal structure. The DFT part of calculations have been done by the Vienna Ab-initio Simulation Package (VASP)[1] with projector augmented-wave (PAW) pseudopotential[2,3] and Perdew-Burke-Ernzerhof parametrization of the generalized gradient approximation (GGA-PBE) exchange-correlation functionals[4]. The energy cutoff of the plane-wave basis is set to be 500 eV, and a $\Gamma$-centered $11 \times 11 \times 11$ $K$-point grid is used.

In $Eu_2Ir_2O_7$, the bands near the Fermi energy are mainly from the $t_{2g}$ orbitals with the energy separation between $e_g$ and $t_{2g}$ orbitals as big as 1.5 eV. The Oxygen $p$-bands are located about 3.0 eV below the Fermi energy, with about 0.5 eV separation between $t_{2g}$ bands. The hybridization between $p$ and $t_{2g}$ orbitals are small. Therefore in our tight-binding (TB) model, we only include the correlated $t_{2g}$ orbitals and doesn't consider the $e_g$ and ligand Oxygen-$p$ orbitals.

Since the number of valence electrons is five, in other words, only one hole per Ir site in the $t_{2g}$ sub-shell on average, the Hund's rule coupling term $J_{\mathrm{H}}$ has small effect if we limit our consideration only within the $t_{2g}$ sub-shell. Therefore, we only add on-site Coulomb interaction $U$ term to the TB Hamiltonian to account for the strong Coulomb interaction among $t_{2g}$ orbitals. We also check the effects of Hund's coupling on the phase diagram, see Fig. S2 and discussion in Sec. IV.

After adding the Coulomb interaction $U$ to the TB Hamiltonian, the double-counting term is just a constant number for specific Coulomb interaction $U$ and can be absorbed in the chemical potential. When we compare the total energy between different magnetic orders at the same Coulomb interaction $U$, the double-counting term is the same due to the same local occupation number, that is 5 in $Eu_2Ir_2O_7$, so the double-counting will not cause any problem in our calculations.

There are several reasons why we choose the tight-binding plus unrestricted Hartree-Fock (TB+UHF) method rather than *ab-initio* methods such as DFT+$U$ or DFT+Gutzwiller[5]. (1) The TB+UHF calculation is fast and the self-consistent loop is easy to converge with the Newton's method, and free of double-counting makes it numerically more stable, while DFT+$U$ and DFT+Gutzwiller calculation for non-collinear magnetism with spin-orbit coupling (SOC) is slow and hard to converge; (2) We want to treat the SOC as a variable to see its effect on the magnetic phase diagram, which is much easier to implement in the TB+UHF method; (3) We don't want to impose any constraint on the local density matrices so that any possible multipolar order parameters are allowed to emerge. We also tried to do the similar calculation by *ab-initio* methods using VASP[1] and OpenMX[6], but we found it is very difficult to make the self-consistent loop converge to any configurations other than all-in-all-out. In our TB+UHF method, we have to apply Newton's method to make the calculation converge within reasonable time, which is not possible at the current stage for *ab-initio* codes. Therefore, based on the above reasons we decided to apply the TB+UHF method for the current studies. The total energy per Ir atom of each stable phase has been converged to within 0.01 meV in our calculations.

## II. DEFINITION OF THE LOCAL $XYZ$-COORDINATE AND LOCAL [111] $xyz$-COORDINATE

Fig. S1(c) is the illustration of the tetrahedron formed by four Ir atoms. We define the local $XYZ$-coordinate with respect to the local Oxygen octahedron (along Ir-O bonds) as follows,

Ir1 $(\frac{1}{2},\frac{1}{2},\frac{1}{2})$:

$$X_1(-\frac{2}{3},\frac{1}{3},-\frac{2}{3}), Y_1(\frac{1}{3},-\frac{2}{3},-\frac{2}{3}), Z_1(-\frac{2}{3},-\frac{2}{3},\frac{1}{3}) \quad \text{(S1)}$$

Ir2 $(\frac{1}{4},\frac{1}{4},\frac{1}{2})$:

$$X_2(\frac{2}{3},-\frac{1}{3},-\frac{2}{3}), Y_2(-\frac{1}{3},\frac{2}{3},-\frac{2}{3}), Z_2(\frac{2}{3},\frac{2}{3},\frac{1}{3}) \quad \text{(S2)}$$

Ir3 $(\frac{1}{4},\frac{1}{2},\frac{1}{4})$:

$$X_3(\frac{2}{3},-\frac{2}{3},-\frac{1}{3}), Y_3(\frac{2}{3},\frac{1}{3},\frac{2}{3}), Z_3(-\frac{1}{3},-\frac{2}{3},\frac{2}{3}) \quad \text{(S3)}$$

Ir4 $(\frac{1}{2},\frac{1}{4},\frac{1}{4})$:

$$X_4(-\frac{2}{3},\frac{2}{3},-\frac{1}{3}), Y_4(-\frac{2}{3},-\frac{1}{3},\frac{2}{3}), Z_4(\frac{1}{3},\frac{2}{3},\frac{2}{3}) \quad \text{(S4)}$$

See Fig. S1(d) for the illustration.

The local [111] $xyz$-coordinate is defined as,

$$\begin{aligned} x_R &= -\frac{1}{\sqrt{6}}X_R - \frac{1}{\sqrt{6}}Y_R + \frac{2}{\sqrt{6}}Z_R, \\ y_R &= \frac{1}{\sqrt{2}}X_R - \frac{1}{\sqrt{2}}Y_R, \\ z_R &= \frac{1}{\sqrt{3}}X_R + \frac{1}{\sqrt{3}}Y_R + \frac{1}{\sqrt{3}}Z_R, \end{aligned} \tag{S5}$$

for Ir1 and Ir2, and

$$\begin{aligned} x_R &= -\frac{1}{\sqrt{6}}Y_R - \frac{1}{\sqrt{6}}Z_R + \frac{2}{\sqrt{6}}X_R, \\ y_R &= \frac{1}{\sqrt{2}}Y_R - \frac{1}{\sqrt{2}}Z_R, \\ z_R &= \frac{1}{\sqrt{3}}X_R + \frac{1}{\sqrt{3}}Y_R + \frac{1}{\sqrt{3}}Z_R, \end{aligned} \tag{S6}$$

for Ir3 and Ir4, where $R$ are the indices of Ir sites. See Fig. S1(e) for the illustration.

## III. DEFINITION OF THE SINGLE-PARTICLE TENSOR (MULTIPOLAR) OPERATORS

In orbital space ($l = 1$), we can define 9 irreducible single-particle tensor operators $T^o_{KQ}, K = 0, 1, 2, Q = -K, \cdots, K$:

$$T^o_{00} = \frac{1}{\sqrt{3}}I \tag{S7}$$

$$T^o_{1\pm1} = \frac{1}{\sqrt{2}}l_\pm \tag{S8}$$

$$T^o_{10} = \frac{1}{\sqrt{2}}l_z \tag{S9}$$

$$T^o_{2\pm2} = l^2_\pm \tag{S10}$$

$$T^o_{2\pm1} = \frac{1}{\sqrt{2}}(l_\pm l_z + l_z l_\pm) \tag{S11}$$

$$T^o_{20} = \frac{1}{\sqrt{6}}(3l^2_z - 2) \tag{S12}$$

and in spin space ($s = \frac{1}{2}$), we can define 4 irreducible single-particle tensor operators $T^s_{KQ}, K = 0, 1, Q = -K, \cdots, K$:

$$T^s_{00} = \frac{1}{\sqrt{2}}I \tag{S13}$$

$$T^s_{1\pm1} = \sqrt{2}s_\pm \tag{S14}$$

$$T^s_{10} = \sqrt{2}s_z \tag{S15}$$

where,

$$l_\pm = \mp\frac{1}{\sqrt{2}}(l_x \pm i l_y) \tag{S16}$$

$$s_\pm = \mp\frac{1}{\sqrt{2}}(s_x \pm i s_y) \tag{S17}$$

and $I$ is the identity operator. These operators are defined with respect to the local [111] $xyz$-coordinate for each Ir atom. With spin-orbit coupling (SOC), we can construct 36 irreducible tensor operators in orbital-spin space,

$$T^{KQ}_{K_1K_2} = \sum_{Q_1Q_2} \langle K_1Q_1K_2Q_2 \,|\, KQ\rangle\, T^o_{K_1Q_1} \otimes T^s_{K_2Q_2}, \tag{S18}$$

where $\langle K_1Q_1K_2Q_2 \,|\, KQ\rangle$ are the Clebsch-Gordan coefficients. $T^{KQ}_{K_1K_2}$ are not Hermitian operators, we can construct Hermitian operators $O^{KM}_{K_1K_2}$ by,

$$O^{KM}_{K_1K_2} = \begin{cases} \frac{1}{\sqrt{2}}\left(T^{K-|Q|}_{K_1K_2} + (-1)^{|Q|}T^{K|Q|}_{K_1K_2}\right) & (|Q| \neq 0, M = |Q|), \\ \frac{i}{\sqrt{2}}\left(T^{K-|Q|}_{K_1K_2} - (-1)^{|Q|}T^{K|Q|}_{K_1K_2}\right) & (|Q| \neq 0, M = |Q| + K), \\ T^{K|Q|}_{K_1K_2} & (|Q| = 0, M = 2K + 1), \end{cases} \tag{S19}$$

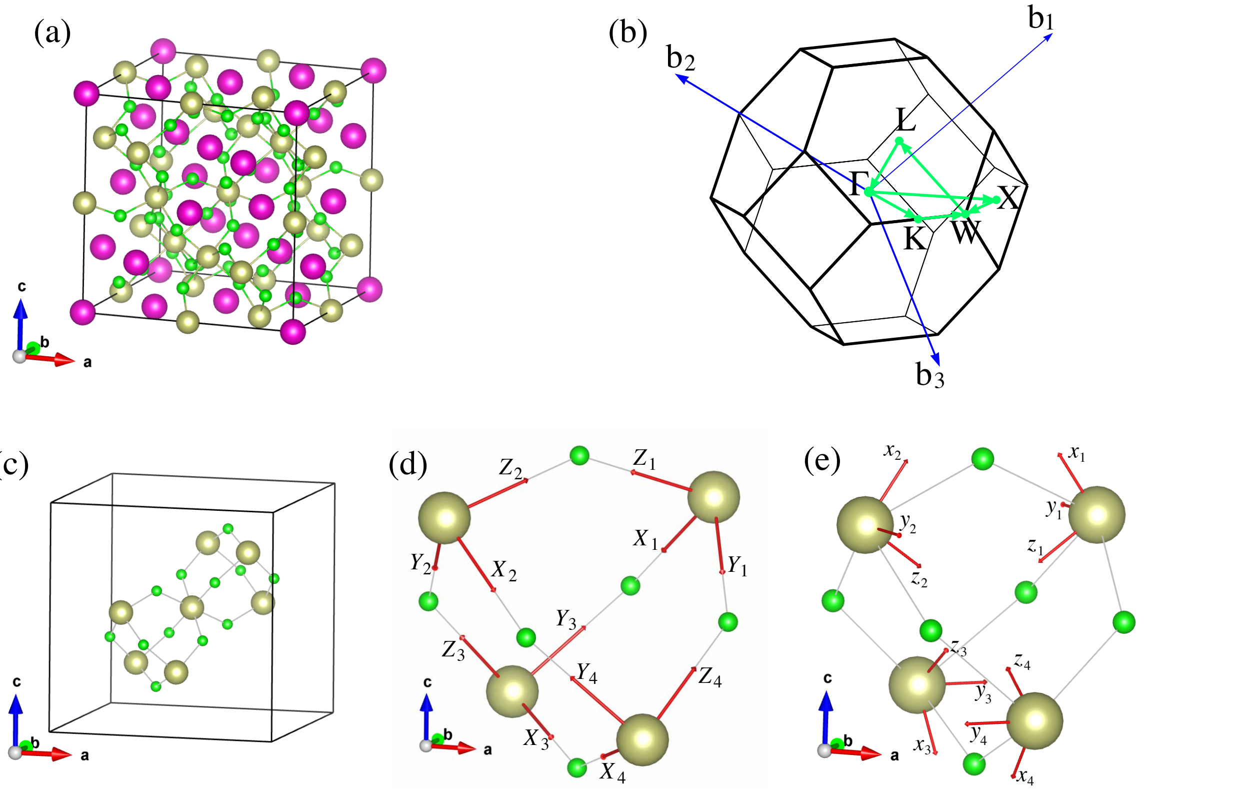


FIG. S1. (Color online). (a) The crystal structure of $Eu_2Ir_2O_7$. (b) The Brillouin zone and high-symmetry $k$-paths. (c) Illustration of the tetrahedron formed by four Ir atoms in $Eu_2Ir_2O_7$. (d) Illustration of the local $XYZ$-coordinate defined along the Ir-O bonds. (e) Illustration of the local [111] $xyz$-coordinate, i.e., $z$-axis is along the local [111] direction.

or

$$O_{K_1K_2}^{KM} = \begin{cases} \frac{-i}{\sqrt{2}}\left(T_{K_1K_2}^{K-|Q|} + (-1)^{|Q|}T_{K_1K_2}^{K|Q|}\right) & (|Q| \neq 0, M = |Q|), \\ \frac{1}{\sqrt{2}}\left(T_{K_1K_2}^{K-|Q|} - (-1)^{|Q|}T_{K_1K_2}^{K|Q|}\right) & (|Q| \neq 0, M = |Q| + K), \\ -iT_{K_1K_2}^{K|Q|} & (|Q| = 0, M = 2K+1), \end{cases} \tag{S20}$$

where, $M = 1, \cdots, 2K+1$. For $K = 1$, indices $M = 1, 2, 3$ serve as the Cartesian $x, y, z$ components, respectively.

All the operators are orthonormal in terms of the inner trace,

$$\mathrm{Tr}\left[O_{K_1K_2}^{KM}\left(O_{K_1'K_2'}^{K'M'}\right)^\dagger\right] = \delta_{K_1K_1'}\delta_{K_2K_2'}\delta_{KK'}\delta_{MM'}. \tag{S21}$$

These 36 irreducible tensor operators form a complete operator basis in the $l = 1, s = \frac{1}{2}$ Hilbert space, and the local density matrix $\rho$ can be expanded in terms of them,

$$\rho = \sum_{K_1K_2KM} C_{K_1K_2}^{KM} O_{K_1K_2}^{KM}, \tag{S22}$$

$$C_{K_1K_2}^{KM} = \mathrm{Tr}\left[\rho\left(O_{K_1K_2}^{KM}\right)^\dagger\right]. \tag{S23}$$

We list them as following:

$$O_{00}^{01} = \frac{1}{\sqrt{6}} I \tag{S24}$$

$$O_{10}^{11} = \frac{1}{2} l_x \tag{S25}$$

$$O_{10}^{12} = \frac{1}{2} l_y \tag{S26}$$

$$O_{10}^{13} = \frac{1}{2} l_z \tag{S27}$$

$$O_{20}^{21} = \frac{1}{2}\left(l_x l_z + l_z l_x\right) \tag{S28}$$

$$O_{20}^{22} = \frac{1}{2}\left(l_x^2 - l_y^2\right) \tag{S29}$$

$$O_{20}^{23} = \frac{1}{2}\left(l_y l_z + l_z l_y\right) \tag{S30}$$

$$O_{20}^{24} = \frac{1}{2}\left(l_x l_y + l_y l_x\right) \tag{S31}$$

$$O_{20}^{25} = \frac{1}{\sqrt{12}}\left(3l_z^2 - 2\right) \tag{S32}$$

$$O_{01}^{11} = \sqrt{\frac{2}{3}} s_x \tag{S33}$$

$$O_{01}^{12} = \sqrt{\frac{2}{3}} s_y \tag{S34}$$

$$O_{01}^{13} = \sqrt{\frac{2}{3}} s_z \tag{S35}$$

$$O_{11}^{01} = -\frac{1}{\sqrt{3}}\left(l_x s_x + l_y s_y + l_z s_z\right) \tag{S36}$$

$$O_{11}^{11} = \frac{1}{\sqrt{2}}\left(l_y s_z - l_z s_y\right) \tag{S37}$$

$$O_{11}^{12} = \frac{1}{\sqrt{2}}\left(l_z s_x - l_x s_z\right) \tag{S38}$$

$$O_{11}^{13} = \frac{1}{\sqrt{2}}\left(l_x s_y - l_y s_x\right) \tag{S39}$$

$$O_{11}^{21} = \frac{1}{\sqrt{2}}\left(l_x s_z + l_z s_x\right) \tag{S40}$$

$$O_{11}^{22} = \frac{1}{\sqrt{2}}\left(l_x s_x - l_y s_y\right) \tag{S41}$$

$$O_{11}^{23} = \frac{1}{\sqrt{2}}\left(l_y s_z + l_z s_y\right) \tag{S42}$$

$$O_{11}^{24} = \frac{1}{\sqrt{2}}\left(l_x s_y + l_y s_x\right) \tag{S43}$$

$$O_{11}^{25} = \frac{1}{\sqrt{6}}\left(2l_z s_z - l_x s_x - l_y s_y\right) \tag{S44}$$

$$\begin{aligned} O_{21}^{11} = \sqrt{\frac{8}{15}}[s_x - \frac{3}{4}((l_x l_y + l_y l_x)s_y \\ +(l_x l_z + l_z l_x)s_z + 2l_x^2 s_x)] \end{aligned} \tag{S45}$$

$$\begin{aligned} O_{21}^{12} = \sqrt{\frac{8}{15}}[s_y - \frac{3}{4}((l_x l_y + l_y l_x)s_x \\ +(l_y l_z + l_z l_y)s_z + 2l_y^2 s_y)] \end{aligned} \tag{S46}$$

$$\begin{aligned} O_{21}^{13} = \sqrt{\frac{8}{15}}[s_z - \frac{3}{4}((l_x l_z + l_z l_x)s_x \\ +(l_y l_z + l_z l_y)s_y + 2l_z^2 s_z)] \end{aligned} \tag{S47}$$

$$\begin{aligned} O_{21}^{21} = -\sqrt{\frac{1}{6}}\left[\left(3l_z^2 - 2\right)s_y - \left(l_y l_z + l_z l_y\right)s_z\right] \\ +\sqrt{\frac{1}{6}}\left[\left(l_x^2 - l_y^2\right)s_y - \left(l_x l_y + l_y l_x\right)s_x\right] \end{aligned} \tag{S48}$$

$$\begin{aligned} O_{2,1}^{22} = -\sqrt{\frac{1}{6}}\left[\left(l_y l_z + l_z l_y\right)s_x + \left(l_x l_z + l_z l_x\right)s_y\right] \\ +\sqrt{\frac{2}{3}}\left(l_x l_y + l_y l_x\right)s_z \end{aligned} \tag{S49}$$

$$\begin{aligned} O_{21}^{23} = \sqrt{\frac{1}{6}}\left[\left(3l_z^2 - 2\right)s_x - \left(l_x l_z + l_z l_x\right)s_z\right] \\ +\sqrt{\frac{1}{6}}\left[\left(l_x^2 - l_y^2\right)s_x + \left(l_x l_y + l_y l_x\right)s_y\right] \end{aligned} \tag{S50}$$

$$\begin{aligned} O_{21}^{24} = \sqrt{\frac{1}{6}}\left[\left(l_x l_z + l_z l_x\right)s_x - \left(l_y l_z + l_z l_y\right)s_y\right] \\ -\sqrt{\frac{2}{3}}\left(l_x^2 - l_y^2\right)s_z \end{aligned} \tag{S51}$$

$$O_{21}^{25} = \sqrt{\frac{1}{2}}\left[\left(l_x l_z + l_z l_x\right)s_y - \left(l_y l_z + l_z l_y\right)s_x\right] \tag{S52}$$

$$\begin{aligned} O_{21}^{31} = \sqrt{\frac{2}{15}}\left(3l_z^2 - 2\right)s_x + \sqrt{\frac{8}{15}}\left(l_x l_z + l_z l_x\right)s_z \\ -\sqrt{\frac{1}{30}}\left[\left(l_x^2 - l_y^2\right)s_x + \left(l_x l_y + l_y l_x\right)s_y\right] \end{aligned} \tag{S53}$$

$$\begin{aligned} O_{21}^{32} = \sqrt{\frac{1}{3}}\left[\left(l_x l_z + l_z l_x\right)s_x - \left(l_y l_z + l_z l_y\right)s_y\right] \\ +\sqrt{\frac{1}{3}}\left(l_x^2 - l_y^2\right)s_z \end{aligned} \tag{S54}$$

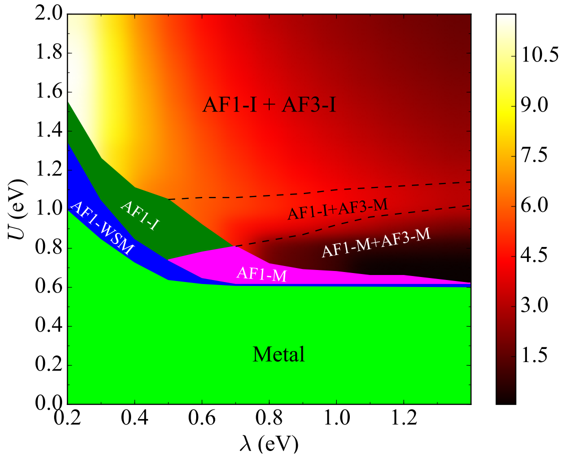


FIG. S2. (Color online). The $U$-$\lambda$ phase diagram for the distorted crystal structure with Hund's coupling $J_{\mathrm{H}}/U = 0.2$.

$$O_{21}^{33} = \sqrt{\frac{1}{2}}\left[\left(l_x^2 - l_y^2\right)s_x - \left(l_x l_y + l_y l_x\right)s_y\right] \quad \text{(S55)}$$

$$O_{21}^{34} = \sqrt{\frac{2}{15}}\left(3l_z^2 - 2\right)s_y + \sqrt{\frac{8}{15}}\left(l_y l_z + l_z l_y\right)s_z + \sqrt{\frac{1}{30}}\left[\left(l_x^2 - l_y^2\right)s_y - \left(l_x l_y + l_y l_x\right)s_x\right] \quad \text{(S56)}$$

$$O_{21}^{35} = \sqrt{\frac{1}{3}}\left[\left(l_y l_z + l_z l_y\right)s_x + \left(l_x l_z + l_z l_x\right)s_y\right] + \sqrt{\frac{1}{3}}\left(l_x l_y + l_y l_x\right)s_z \quad \text{(S57)}$$

$$O_{21}^{36} = \sqrt{\frac{1}{2}}\left[\left(l_x^2 - l_y^2\right)s_y + \left(l_x l_y + l_y l_x\right)s_x\right] \quad \text{(S58)}$$

$$O_{21}^{37} = -\sqrt{\frac{1}{5}}\left[\left(l_x l_z + l_z l_x\right)s_x + \left(l_y l_z + l_z l_y\right)s_y\right] + \sqrt{\frac{1}{5}}\left(3l_z^2 - 2\right)s_z \quad \text{(S59)}$$

## IV. PHASE DIAGRAM WITH HUND'S COUPLING

To check the effect of Hund's coupling $J_{\mathrm{H}}$ on the magnetic states, we calculate the phase diagram for the distorted crystal structure with Hund's coupling $J_{\mathrm{H}}/U = 0.2$, which is shown in Fig. S2. Hund's coupling doesn't change the overall phase diagram and it only shifts the position of phase boundary. This is reasonable because there is only one hole per Ir site in $t_{2g}$ bands and the Hund's coupling will not play significant role here.

## V. BAND STRUCTURES

We pick several representative points for each phase from the phase diagram in Fig. 2(a,b) in the main text to plot their band structures, which are shown in Fig. S3 and Fig. S4. Fig. S3 is for the distorted crystal structure and Fig. S4 is for the non-distorted crystal structure.

Fig. S3(a,b,c,d) and Fig. S4(a,b,c,d) are band structures for paramagnetic metal phase at small $U$ (=0.3 eV). Due to SOC, the bands are splitted into two parts, the half-filled $j_{\mathrm{eff}} = 1/2$ bands with higher energy and the fully-filled $j_{\mathrm{eff}} = 3/2$ bands with lower energy. At $\Gamma$ point, there is a quadratic band touch near Fermi level in the $j_{\mathrm{eff}} = 1/2$ bands, which is also observed in $Pr_2Ir_2O_7$[7] and $Nd_2Ir_2O_7$[8] by ARPES. At small SOC, the degeneracies of eight $j_{\mathrm{eff}} = 1/2$ bands have a "2-4-2" band order (in order of increasing energy). With the increment of SOC, the quadratic touch point is pushed down to have a band inversion, and the band order is changed to "4-2-2". After the band inversion, if a global gap is open, then it becomes a topological insulator (TI). This is the case for the non-distorted crystal structure and is similar to results in Ref. 9, while it is still metallic phase for the distorted crystal structure at very large SOC (1.4 eV for example).

For distorted crystal structure, at $\lambda = 0.4$ eV and after increasing $U$ to about 0.6 eV, it first changes to AF1 Weyl semimetal phase (Fig. S3(e)), then changes to AF1 insulator phase (Fig. S3(f)), and finally to the insulating phase where AF1 (Fig. S3(g)) and AF3 (Fig. S3(h)) coexist. This semimetal-to-insualtor transition is similar to that in $Y_2Ir_2O_7$[10]. Fig. S3(e) is the band structure for Weyl semimetal phase, the Weyl point is far away from the high-symmetry lines of $k$ points, which is also the case in $Y_2Ir_2O_7$[10]. Note that it is not a real band cross in the inset figure. At the reasonable parameters $\lambda = 0.4$ eV and $U = 1.1$ eV we choose for $Eu_2Ir_2O_7$, the AF1 phase has a band gap of about 0.4 eV (Fig. S3(g)) and the AF3 phase has a band gap of about 0.35 eV (Fig. S3(h)), which are little larger than the optical gap (0.2 eV) reported in Ref. 11 and the gap (0.3 eV) produced by the LDA+DMFT calculations[12]. This is reasonable considering the fact that Hartree-Fock calculations usually overestimate the band gaps. Fig. S3(i,j,k,l) are band structures for distorted crystal structure at $\lambda = 0.8$ eV. When $U$ is small (0.6 eV), both AF1 (Fig. S3(i)) and AF3 (Fig. S3(j)) are metallic phase, while they change to insulator phase (Fig. S3(k) for AF1 and Fig. S3(l) for AF3) at larger $U$ (1.1 eV)

For non-distorted crystal structure, at $\lambda = 0.4$ eV and after $U$ is increased to large value (for example $U = 1.4$ eV), AF1 (Fig. S4(f)), AF2 (Fig. S4(g)) and AF3 (Fig. S4(h)) insulating phases coexist. At $\lambda = 1.0$ eV, only AF2 insulator phase (Fig. S4(i)) is stable when $U$ is small (1.4 eV), while AF2 insulator phase (Fig. S4(j)) and AF3 insulator phase (Fig. S4(k)) coexist at larger $U$ (1.8 eV). In Ref. 9, they also found a AF2 phase in the $U$-$t_\sigma$ phase diagram. Fig. S4(l) is the band struc-

ture for AF1 Weyl semimetal phase at $\lambda = 0.2$ eV and $U = 1.3$ eV, where the Weyl points are along $\Gamma - L$, the high-symmetry lines of $k$ points. For Weyl semimetal phase, we find that whether the Weyl points are along high-symmetry lines of $k$ points or not depends on the parameters $\lambda$ and $U$.


1 G. Kresse and J. Furthmüller, Phys. Rev. B **54**, 11169 (1996).

2 P. E. Blöchl, Phys. Rev. B **50**, 17953 (1994).

3 G. Kresse and D. Joubert, Phys. Rev. B **59**, 1758 (1999).

4 J. P. Perdew, K. Burke, and M. Ernzerhof, Phys. Rev. Lett. **77**, 3865 (1996).

5 X. Y. Deng, L. Wang, X. Dai, and Z. Fang, Phys. Rev. B **79**, 075114 (2009).

6 The *OpenMX* code is available at `http://www.openmx-square.org/`.

7 T. Kondo, M. Nakayama, R. Chen, J. J. Ishikawa, E.-G. Moon, T. Yamamoto, Y. Ota, W. Malaeb, H. Kanai, Y. Nakashima, Y. Ishida, R. Yoshida, H. Yamamoto, M. Matsunami, S. Kimura, N. Inami, K. Ono, H. Kumigashira, S. Nakatsuji, L. Balents, and S. Shin, Nat. Comm. **6**, 10042 (2015).

8 M. Nakayama, T. Kondo, Z. Tian, J. J. Ishikawa, M. Halim, C. Bareille, W. Malaeb, K. Kuroda, T. Tomita, S. Ideta, K. Tanaka, M. Matsunami, S. Kimura, N. Inami, K. Ono, H. Kumigashira, L. Balents, S. Nakatsuji, and S. Shin, Phys. Rev. Lett. **117**, 056403 (2016).

9 W. Witczak-Krempa and Y. B. Kim, Phys. Rev. B **85**, 045124 (2012).

10 X. Wan, A. M. Turner, A. Vishwanath, and S. Y. Savrasov, Phys. Rev. B **83**, 205101 (2011).

11 K. Ueda, J. Fujioka, and Y. Tokura, Phys. Rev. B **93**, 245120 (2016).

12 H. Zhang, K. Haule, and D. Vanderbilt, Phys. Rev. Lett. **118**, 026404 (2017).

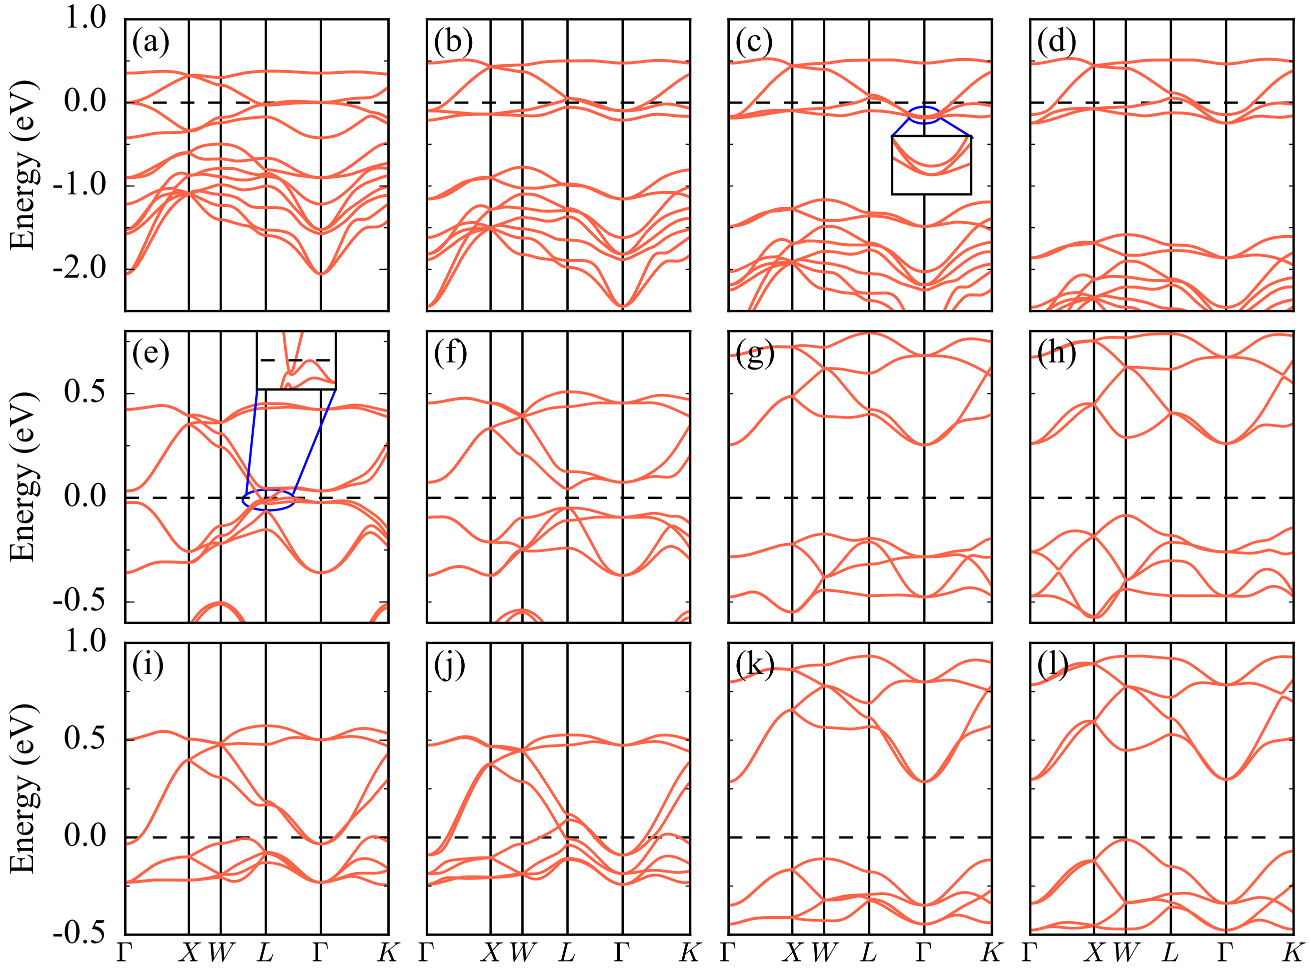


FIG. S3. (Color online). Band structures for the distorted crystal structure. (a) $\lambda = 0.4$ eV, $U = 0.3$ eV, paramagnetic metal. (b) $\lambda = 0.8$ eV, $U = 0.3$ eV, paramagnetic metal. (c) $\lambda = 1.1$ eV, $U = 0.3$ eV, paramagnetic metal, note that there is a band inversion at Γ point. (d) $\lambda = 1.4$ eV, $U = 0.3$ eV. paramagnetic metal. (e) $\lambda = 0.4$ eV, $U = 0.6$ eV, AF1 Weyl semimetal, note that there is no Weyl point in the inset figure and the Weyl points are far away from the high-symmetry $k$ points. (f) $\lambda = 0.4$ eV, $U = 0.7$ eV, AF1 insulator. (g) $\lambda = 0.4$ eV, $U = 1.1$ eV, AF1 insulator. (h) $\lambda = 0.4$ eV, $U = 1.1$ eV, AF3(A) insulator. (i) $\lambda = 0.8$ eV, $U = 0.6$ eV, AF1 metal. (j) $\lambda = 0.8$, $U = 0.6$ eV, AF3(A) metal. (k) $\lambda = 0.8$ eV, $U = 1.1$ eV, AF1 insulator. (l) $\lambda = 0.8$ eV, $U = 1.1$ eV, AF3(A) insulator.

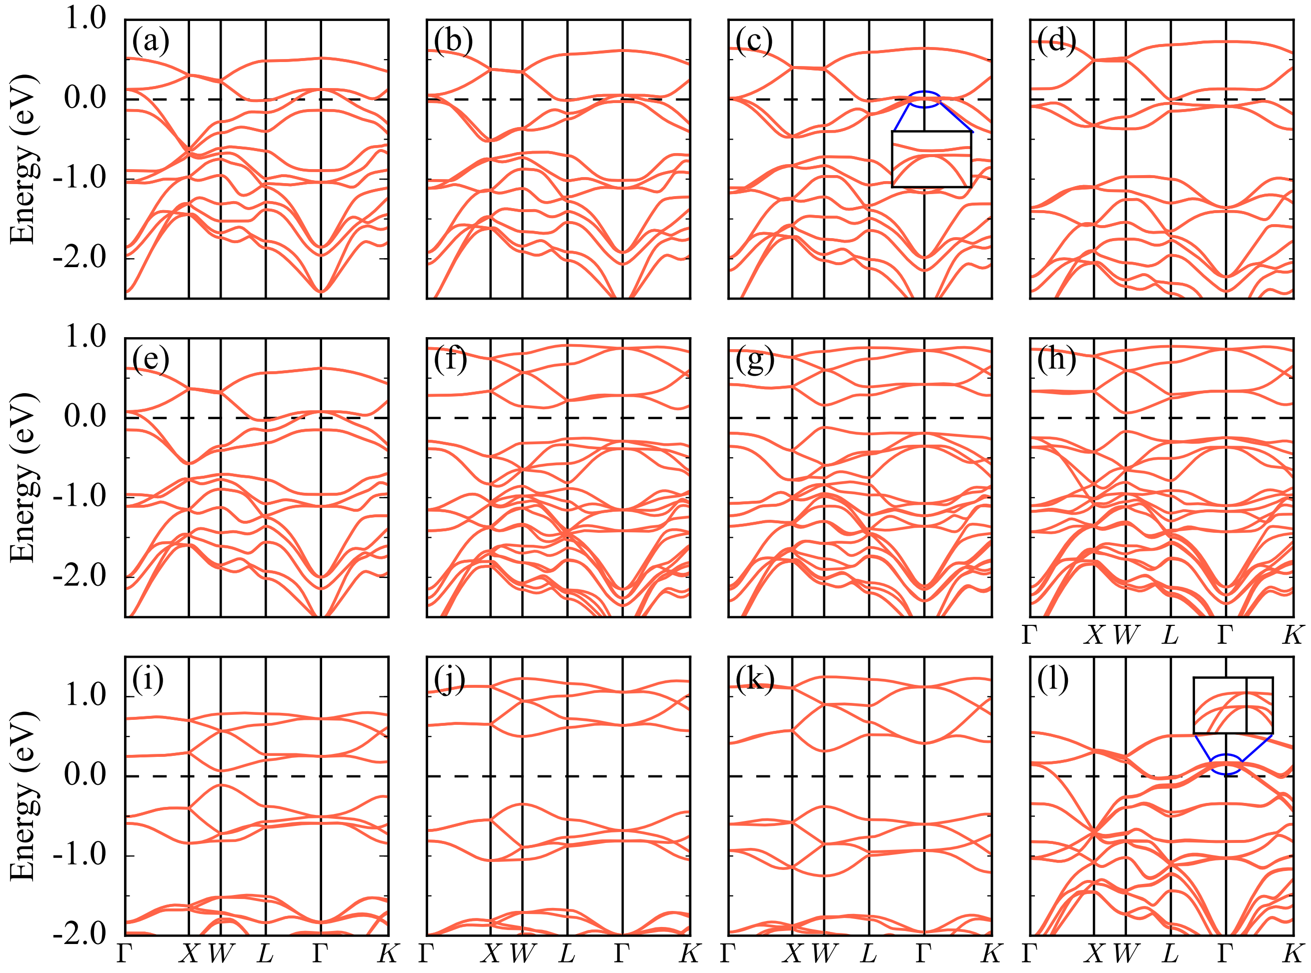


FIG. S4. (Color online). Band structures for the non-distorted crystal structure ($x = 5/16$). (a) $\lambda = 0.4$ eV, $U = 0.3$ eV, paramagnetic metal. (b) $\lambda = 0.6$ eV, $U = 0.3$ eV, paramagnetic metal. (c) $\lambda = 0.7$ eV, $U = 0.3$ eV, paramagnetic metal, note that there is a band inversion at Γ point. (d) $\lambda = 1.0$ eV, $U = 0.3$ eV, gap opens, it is a topological insulator. (e) $\lambda = 0.4$ eV, $U = 1.0$ eV, paramagnetic metal. (f) $\lambda = 0.4$ eV, $U = 1.4$ eV, AF1 insulator. (g) $\lambda = 0.4$ eV, $U = 1.4$ eV, AF2(B) insulator. (h) $\lambda = 0.4$ eV, $U = 1.4$ eV, AF3(A) insulator. (i) $\lambda = 1.0$ eV, $U = 1.2$ eV, AF2(B) insulator. (j) $\lambda = 1.0$,eV, $U = 1.8$ eV, AF2(B) insulator. (k) $\lambda = 1.0$ eV, $U = 1.8$ eV, AF3(A) insulator. (l) $\lambda = 0.2$ eV, $U = 1.3$ eV, AF1 Weyl semimetal, see the inset figure, there is a Weyl point along Γ-$L$ line.
